# Supplementary material for: Automating Safety and Security Co-Design through Semantically-Rich Architecture Patterns
Source: arXiv:2201.10563 source file (2022-02-27)
Supplement: Supplementary file 1 [file appendix.tex]

%!TEX root = tcps21.tex
\section*{Appendix}

This appendix contains the specification of further safety and security patterns that are not described to the article \emph{NAME OF THE ARTICLE}.

\subsection*{Specification of Safety Patterns}
The heterogeneous duplex pattern with fail safe consists of a primary and a secondary (a.k.a. redundant) component, and a fault detector.
The primary and secondary components have different design implementations and operate in parallel.
%The fault detector receives the inputs as for the primary and secondary components. 
The fault detector consumes the computations from the primary and secondary components and their original inputs such that it can cross-check their computations to identify failures of type erroneous.
While no failure is detected by the fault detector (\eg, through the use of plausibility checks), the actuator receives the outputs from the primary component. 
If the fault detector identifies a failure on the primary component, the fault detector ensures that the actuator will receive the outputs from the secondary component instead. 
This pattern fails operational always after the 1st failure of type erroneous (\ie, failure on the primary component), and it transition the system to a safe state whenever the secondary failure is detected (\ie, failure on the secondary component). This pattern never fails silent.
The instantiation of the heterogeneous duplex pattern with fail safe pattern is shown in Table~\ref{table:htd-with-fs}. 

\begin{table}[h]
\centering
\begin{tabular}[t]{p{2cm}p{5.5cm}p{5.5cm}}
%\begin{tabularx}{\textwidth}{lcc}
\toprule
&Description &\machinery Specification\\
\midrule
Pattern name&Heterogeneous Duplex Pattern with Fail Safe&\code{NAME=heterogeneousDuplexFS;}\\
\hline
Other well-known names&Heterogeneous Redundancy Pattern, Diverse Redundancy Pattern&\\
\hline
Structure&\begin{minipage}{.3\textwidth}\includegraphics[scale=0.35]{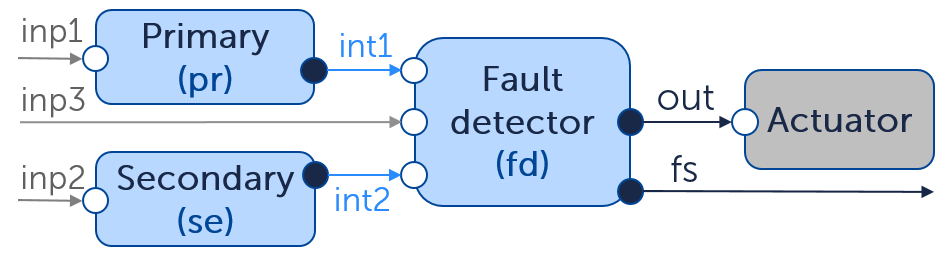}\end{minipage}
&
%\vspace*{-1cm}
%\begin{minipage}
%{.3\textwidth}
%\code{ID=PAT;}
%\code{PRIMARY=PR;}                                      
\code{COMPONENTS=[PR,SE,FD];} 
%\code{FAULT\_DETECTOR=FD;} 
\code{INPUT\_CH=[inp1,inp2,inp3];} 
\code{INTERNAL\_CH=[int1,int2];}
\code{OUTPUT\_CH=[out,fs];}
%\code{FAIL\_SAFE=fs;}
%\code{OUTPUT\_CH\_FS=[out\_fs];}
%\end{minipage}
\\
\hline
Intent&This pattern is suitable for high criticality hazards (ASIL C and D)~\cite{Armoush2010}. This pattern fails operational \red{always after the 1st} erroneous failure, and it transition the system to a safe state always after the 2nd failure has been detected. This pattern never fails silent.&
%\begin{tabular}{l}
\code{TYPE\_FAIL=[err];} 
\code{ASIL=d;}                                      
\code{FAIL\_OP=all1fail;} 
\code{FAIL\_SILENT=never;}
%\code{FAIL\_SAFE=on\_2fail;}
%\code{FAIL\_SAFE=true;} 
\code{FAIL\_SAFE=all2fail;}
%\end{tabular}
\\
%\hline
Problem addressed&This pattern tolerates faults by avoiding failures of type erroneous.&\\
\hline
Assumptions&The primary and secondary components shall be implemented using independent designs. &\code{TYPE\_ASSUMPTION=are\_independent;}
\code{COMPONENT={[PR,SE]};}\\\cdashline{2-3}
&The primary and the secondary component shall be allocated to dedicated hardware units. &\code{TYPE\_ASSUMPTION=are\_decoupled;}
\code{COMPONENT={[PR,SE]};}\\\cdashline{2-3}
%& The primary and secondary component shall implement a BIT for loss detection. &\code{TYPE\_ASSUMPTION=have\_BIT\_loss;}
%\code{COMPONENT={[PR,SE]};}\\\cdashline{2-3}
& The fault detector shall be verified. &\code{TYPE\_ASSUMPTION=are\_verified;}
\code{COMPONENT={[FD]};}\\\cdashline{2-3}
\hline
Consequences (security)&There is a potential threat associated with the fault detector. That is, as an attacker may carry out malicious actions to prevent the fault detector from properly functioning. This potential threat is of type \textbf{int}egrity if the failure associated with the primary component is of type erroneous. &
%\code{ID\_THREAT=ID;}
\code{COMPONENT=FD;}
\code{TYPE\_THREAT=int;}
%\code{SEVERITY\_THREAT=sev;} 
\\
\bottomrule
\end{tabular}
\caption{Heterogeneous duplex pattern with fail safe}
\label{table:htd-with-fs}
\end{table}%

%\subsubsection{Specification in SafSecPat}

We describe the specification of the heterogeneous duplex pattern with fail safe in \machinery.
Consider the language for safety patterns described in Table~\ref{table:dsl-safsecpat} and the structure of the pattern illustrated in Table~\ref{table:htd-with-fs}. 
This pattern is instantiated as follows:
\begin{center}
\code{safetyPattern(idpat,[heterogeneousDuplexFS,[pr,se,fd],
     [inp1,inp2,inp3],[int1,int2],[out,fs]]).}
\end{center}
